# Supplementary material for: Towards the quantum exceptional series
Source: arXiv:2402.03637 source file (2025-04-08)
Supplement: Supplementary file 1 [file AppendixCalculations.pdf]

In[•]:=
```
(*This file checks the calculations of the coefficients on the square relation, given in the appendix of the main paper.*)
```

In[•]:=
```
SquareRelation = {(-1 + v^6)/v^3, 0, 0, α (b v + α - v (t + v α))/v, 0, (-1 + v^2) (-t v + (1 + v^4 + v^6) α)/v^2,
  -(-1 + v^2) (t v^5 + (1 + v^2 + v^6) α)/v^6, α (-t v + b v^3 + α - v^2 α)/v^5, v^2 α (b + v (α - v (t + v α)))}
```

Out[•]=
$$\left\{\frac{-1+v^6}{v^3},0,0,\frac{\alpha\left(b\,v+\alpha-v\,(t+v\,\alpha)\right)}{v},0,\frac{\left(-1+v^2\right)\left(-t\,v+\left(1+v^4+v^6\right)\alpha\right)}{v^2},-\frac{\left(-1+v^2\right)\left(t\,v^5+\left(1+v^2+v^6\right)\alpha\right)}{v^6},\frac{\alpha\left(-t\,v+b\,v^3+\alpha-v^2\alpha\right)}{v^5},v^2\alpha\left(b+v\,(\alpha-v\,(t+v\,\alpha))\right)\right\}$$

In[•]:=
```
NormalizedSquareRelation =
  FullSimplify[SquareRelation / SquareRelation[[1]] /. t → (b - (v^5 - v^-5) α)/(v^2 + v^-2)]
```

Out[•]=
$$\left\{1,0,0,\frac{\left(1-v^2+v^4\right)\alpha\left(b\,v^3+\left(-1+v^6\right)\alpha\right)}{\left(1+v^4\right)\left(-1+v^6\right)},0,\frac{-b\,v^5-\alpha+v^2\alpha+v^6\left(2+v^2\right)\left(1+v^4\right)\alpha}{v\left(1+v^4\right)\left(1+v^2+v^4\right)},-\frac{\left(-1+v^2\right)\left(\left(1+v^2+v^6\right)\alpha+\frac{v^2\left(b\,v^5+\alpha-v^{10}\alpha\right)}{1+v^4}\right)}{v^3\left(-1+v^6\right)},\frac{\alpha\left(b\,v^9-\alpha+v^2\alpha+(-1+v)\,v^4\,(1+v)\left(1+v^4\right)\alpha\right)}{v^4\left(1+v^4\right)\left(-1+v^6\right)},\frac{v^4\alpha\left(-\alpha+v\left(b+v\,\alpha+(-1+v)\,v^3\,(1+v)\left(1+v^4\right)\alpha\right)\right)}{\left(1+v^4\right)\left(-1+v^6\right)}\right\}$$

In[•]:=

In[•]:=
```
Psi[n_, v_] := v^-EulerPhi[n] Cyclotomic[n, v^2]
```

In[•]:=
```
FullSimplify[NormalizedSquareRelation[[4]] / ((α Psi[6, v] (b + (v^3 - v^-3) α))/(Psi[1, v] × Psi[3, v] × Psi[4, v]))]
```

Out[•]= 1

In[•]:=
```
Collect[Expand[NormalizedSquareRelation[[6]] Psi[3, v] × Psi[4, v]], α]
```

Out[•]=
$$-b+\left(-\frac{1}{v^5}+\frac{1}{v^3}+2\,v+v^3+2\,v^5+v^7\right)\alpha$$

In[•]:=
```
FullSimplify[NormalizedSquareRelation[[7]] Psi[3, v] × Psi[4, v] ]
```

Out[•]=
$$-b+\frac{\left(-1-2\,v^2-v^4-2\,v^6-v^{10}+v^{12}\right)\alpha}{v^7}$$

In[•]:=
```
FullSimplify[NormalizedSquareRelation[[8]] Psi[1, v] × Psi[3, v] × Psi[4, v] / α]
```

Out[•]=
$$b+\frac{\left(-1+v^2-v^4+v^6-v^8+v^{10}\right)\alpha}{v^9}$$

In[•]:= `FullSimplify[NormalizedSquareRelation[[9]] Psi[1, v] × Psi[3, v] × Psi[4, v] / α]`

Out[•]= $b + \frac{\left(-1 + v^2 - v^4 + v^6 - v^8 + v^{10}\right)\alpha}{v}$

In[•]:= $\text{bRule} = b \to \frac{\left(w\,v^2 + w^{-1}\,v^{-2}\right)\left(w\,v^{-3} + w^{-1}\,v^3\right)\left(v^3 - v^{-3}\right)}{v - v^{-1}}$

$b \to \frac{\left(-\frac{1}{v^3} + v^3\right)\left(\frac{v^3}{w} + \frac{w}{v^3}\right)\left(\frac{1}{v^2 w} + v^2 w\right)}{-\frac{1}{v} + v}$

$\alpha\text{Rule} = \alpha \to -\frac{\left(w - w^{-1}\right)\left(w\,v^{-1} - w^{-1}\,v\right)}{v - v^{-1}}$

$\alpha \to -\frac{\left(-\frac{1}{w} + w\right)\left(-\frac{v}{w} + \frac{w}{v}\right)}{-\frac{1}{v} + v}$

$\text{tRule} = t \to \left(v + v^{-1}\right)\left(\left(v + v^{-1}\right)\frac{w^2}{v} + \left(v^4 - v^2 - 1 - v^{-2} + v^{-4}\right) + \left(v + v^{-1}\right)\frac{v}{w^2}\right)$

$t \to \left(\frac{1}{v} + v\right)\left(-1 + \frac{1}{v^4} - \frac{1}{v^2} - v^2 + v^4 + \frac{v\left(\frac{1}{v} + v\right)}{w^2} + \frac{\left(\frac{1}{v} + v\right)w^2}{v}\right)$

$\text{dRule} = d \to -\frac{\left(v^2 + v^{-2}\right)\left(w\,v^5 - w^{-1}\,v^{-5}\right)\left(w\,v^{-6} - w^{-1}\,v^6\right)}{\left(w - w^{-1}\right)\left(w\,v^{-1} - w^{-1}\,v\right)}$

$d \to -\frac{\left(\frac{1}{v^2} + v^2\right)\left(-\frac{v^6}{w} + \frac{w}{v^6}\right)\left(-\frac{1}{v^5 w} + v^5 w\right)}{\left(-\frac{1}{w} + w\right)\left(-\frac{v}{w} + \frac{w}{v}\right)}$

Out[•]= $b \to \frac{\left(-\frac{1}{v^3} + v^3\right)\left(\frac{v^3}{w} + \frac{w}{v^3}\right)\left(\frac{1}{v^2 w} + v^2 w\right)}{-\frac{1}{v} + v}$

Out[•]= $b \to \frac{\left(-\frac{1}{v^3} + v^3\right)\left(\frac{v^3}{w} + \frac{w}{v^3}\right)\left(\frac{1}{v^2 w} + v^2 w\right)}{-\frac{1}{v} + v}$

Out[•]= $\alpha \to -\frac{\left(-\frac{1}{w} + w\right)\left(-\frac{v}{w} + \frac{w}{v}\right)}{-\frac{1}{v} + v}$

Out[•]= $\alpha \to -\frac{\left(-\frac{1}{w} + w\right)\left(-\frac{v}{w} + \frac{w}{v}\right)}{-\frac{1}{v} + v}$

Out[•]= $t \to \left(\frac{1}{v} + v\right)\left(-1 + \frac{1}{v^4} - \frac{1}{v^2} - v^2 + v^4 + \frac{v\left(\frac{1}{v} + v\right)}{w^2} + \frac{\left(\frac{1}{v} + v\right)w^2}{v}\right)$

Out[•]= $t \to \left(\frac{1}{v} + v\right)\left(-1 + \frac{1}{v^4} - \frac{1}{v^2} - v^2 + v^4 + \frac{v\left(\frac{1}{v} + v\right)}{w^2} + \frac{\left(\frac{1}{v} + v\right)w^2}{v}\right)$

Out[•]= $d \to -\frac{\left(\frac{1}{v^2}+v^2\right)\left(-\frac{v^6}{w}+\frac{w}{v^6}\right)\left(-\frac{1}{v^5 w}+v^5 w\right)}{\left(-\frac{1}{w}+w\right)\left(-\frac{v}{w}+\frac{w}{v}\right)}$

Out[•]= $d \to -\frac{\left(\frac{1}{v^2}+v^2\right)\left(-\frac{v^6}{w}+\frac{w}{v^6}\right)\left(-\frac{1}{v^5 w}+v^5 w\right)}{\left(-\frac{1}{w}+w\right)\left(-\frac{v}{w}+\frac{w}{v}\right)}$

In[•]:=
```
WVariablesSquareRelation =
  FullSimplify[NormalizedSquareRelation /. bRule /. αRule /. tRule /. dRule]
```

Out[•]= $\Big\{1, 0, 0, \frac{\left(1+v^2\right)\left(1-v^2+v^4\right)^2 (v-w)(v+w)\left(-1+w^2\right)}{v^4\left(-1+v^2\right)^2 w^2},$
$0, \frac{-v^4\left(-1+v^2+v^4\right)+\left(1-2v^2+3v^6\right)w^2-v^2\left(-1+v^2+v^4\right)w^4}{v^3\left(-1+v^2\right)w^2},$
$\frac{v^2+v^4-v^6-v^2\left(3-2v^4+v^6\right)w^2+\left(1+v^2-v^4\right)w^4}{v^3\left(-1+v^2\right)w^2},$
$\frac{(v-w)(v+w)\left(-1+w^2\right)\left(v^2\left(-1+v^2\right)+\left(1+v^2-v^4+v^8\right)w^2+\left(-1+v^2\right)w^4\right)}{v^4\left(-1+v^2\right)^2 w^4},$
$\frac{(v-w)(v+w)\left(-1+w^2\right)\left(w^2+v^8\left(-1+w^2\right)+v^4 w^2\left(-1+w^2\right)+v^6\left(1+w^2-w^4\right)\right)}{v^2\left(-1+v^2\right)^2 w^4}\Big\}$

In[•]:=
```
FullSimplify[
  -WVariablesSquareRelation[[4]] Psi[1, v]^2 / (Psi[2, v] Psi[6, v]^2 (w - w^-1) (w v^-1 - w^-1 v))]
```

Out[•]= 1

In[•]:=
```
Collect[WVariablesSquareRelation[[6]] Psi[1, v], w]
```

Out[•]= $\frac{1-2v^2+3v^6}{v^4}-\frac{-1+v^2+v^4}{w^2}-\frac{\left(-1+v^2+v^4\right)w^2}{v^2}$

In[•]:=
```
(*Checking directly against the paper,
but keeping in mind that mathematica deals with parentheses in TeX wrongly*)
```

In[•]:=
```
ToExpression[
  "w^{-2} (1-v^2-v^4)  + (v^{-4} - 2 v^{-2} + 3 v^2) + w^2 (v^{-2} -1-v^2)",
  TeXForm, HoldForm]
```

Out[•]= $\frac{1}{w^2}\left[1-v^2-v^4\right]+\left(\frac{1}{v^4}-\frac{2}{v^2}+3v^2\right)+w^2\left[\frac{1}{v^2}-1-v^2\right]$

In[•]:=
```
Simplify[WVariablesSquareRelation[[6]] Psi[1, v] ==
   1/w^2 (1 - v^2 - v^4) + (1/v^4 - 2/v^2 + 3 v^2) + w^2 (1/v^2 - 1 - v^2)]
```

Out[•]= True

In[•]:= `Collect[WVariablesSquareRelation[[7]] Psi[1, v], w]`

Out[•]= $-\frac{3-2 v^4+v^6}{v^2}+\frac{v^2+v^4-v^6}{v^4 w^2}+\frac{\left(1+v^2-v^4\right) w^2}{v^4}$

In[•]:= `ToExpression["w^{-2}(v^{-2}+1-v^2)+(-3v^{-2}+2v^2-v^4)+w^2(v^{-4}+v^{-2}-1)", TeXForm, HoldForm]`

Out[•]= $\frac{1}{w^2}\left[\frac{1}{v^2}+1-v^2\right]+\left(-\frac{3}{v^2}+2 v^2-v^4\right)+w^2\left[\frac{1}{v^4}+\frac{1}{v^2}-1\right]$

In[•]:= `Simplify[WVariablesSquareRelation[[7]] Psi[1, v] ==` $\frac{1}{w^2}\left(\frac{1}{v^2}+1-v^2\right)+\left(-\frac{3}{v^2}+2 v^2-v^4\right)+w^2\left(\frac{1}{v^4}+\frac{1}{v^2}-1\right)$`]`

Out[•]= True

In[•]:= `Collect[Expand[WVariablesSquareRelation[[8]] Psi[1, v]^2], w]`

Out[•]= $-1+\frac{1}{v^6}+\frac{4}{v^4}-\frac{2}{v^2}+v^2+v^4+\frac{-1+\frac{1}{v^2}}{w^4}+\frac{2-\frac{2}{v^4}-\frac{1}{v^2}-v^4}{w^2}+\left(-\frac{2}{v^6}-\frac{1}{v^4}+\frac{2}{v^2}-v^2\right) w^2+\left(\frac{1}{v^6}-\frac{1}{v^4}\right) w^4$

In[•]:= 
```
ToExpression["w^{-4} (v^{-2} - 1) +
  w^{-2} (-2 v^{-4} - v^{-2} + 2 - v^4) + (v^{-6} + 4 v^{-4} -
    2 v^{-2} - 1 + v^2 + v^4) +
  w^2 (-2 v^{-6} - v^{-4} + 2 v^{-2} - v^2) + w^4 (v^{-6} - v^{-4})",
  TeXForm, HoldForm]
```

Out[•]= $\frac{1}{w^4}\left[\frac{1}{v^2}-1\right]+\frac{1}{w^2}\left[-\frac{2}{v^4}-\frac{1}{v^2}+2-v^4\right]+\left(\frac{1}{v^6}+\frac{4}{v^4}-\frac{2}{v^2}-1+v^2+v^4\right)+w^2\left[-\frac{2}{v^6}-\frac{1}{v^4}+\frac{2}{v^2}-v^2\right]+w^4\left[\frac{1}{v^6}-\frac{1}{v^4}\right]$

In[•]:= `FullSimplify[WVariablesSquareRelation[[8]] Psi[1, v]^2 ==` $\frac{1}{w^4}\left(\frac{1}{v^2}-1\right)+\frac{1}{w^2}\left(-\frac{2}{v^4}-\frac{1}{v^2}+2-v^4\right)+\left(\frac{1}{v^6}+\frac{4}{v^4}-\frac{2}{v^2}-1+v^2+v^4\right)+w^2\left(-\frac{2}{v^6}-\frac{1}{v^4}+\frac{2}{v^2}-v^2\right)+w^4\left(\frac{1}{v^6}-\frac{1}{v^4}\right)$`]`

Out[•]= True

In[•]:= `Collect[WVariablesSquareRelation[[9]] Psi[1, v]^2, w]`

Out[•]= $\frac{1+v^2-v^4-2 v^6+4 v^8+v^{10}}{v^4}+\frac{-v^8+v^{10}}{v^4 w^4}+\frac{-v^2+2 v^6-v^8-2 v^{10}}{v^4 w^2}+\frac{\left(-1+2 v^4-v^6-2 v^8\right) w^2}{v^4}+\frac{\left(-v^4+v^6\right) w^4}{v^4}$

In[•]:=
```
ToExpression[
  "w^{-4}(-v^4 + v^6) + w^{-2}(-v^{-2}+2v^2-v^4-2v^6) + (v^{-4} + v^{-2}
   -1-2v^2+4v^4+v^6) +w^2 (-v^{-4} +2 -v^2 - 2 v^4)
   + w^4 (-1+v^2)", TeXForm, HoldForm]
```

Out[•]=
$$\frac{1}{w^4}\left[-v^4+v^6\right]+\frac{1}{w^2}\left[-\frac{1}{v^2}+2v^2-v^4-2v^6\right]+\left(\frac{1}{v^4}+\frac{1}{v^2}-1-2v^2+4v^4+v^6\right)+w^2\left[-\frac{1}{v^4}+2-v^2-2v^4\right]+w^4\left[-1+v^2\right]$$

In[•]:=
```
FullSimplify[
  WVariablesSquareRelation[[9]] Psi[1, v]^2 ==
```
$$\frac{1}{w^4}\left(-v^4+v^6\right)+\frac{1}{w^2}\left(-\frac{1}{v^2}+2v^2-v^4-2v^6\right)+\left(\frac{1}{v^4}+\frac{1}{v^2}-1-2v^2+4v^4+v^6\right)+w^2\left(-\frac{1}{v^4}+2-v^2-2v^4\right)+w^4\left(-1+v^2\right)]$$

Out[•]= True
